# Supplementary material for: Formulas for Generalized Two-Qubit Separability Probabilities
Source: arXiv:1609.08561 source file (2017-08-10)
Supplement: Supplementary file 1 [file AdditionalPkaFormulas2.pdf]

$$P\,(-1-4\,\alpha,\,\alpha) = \frac{1}{4}\left(1+\frac{3\times 16^{\alpha}\,\text{Gamma}\left[\frac{1}{2}+2\,\alpha\right]}{\sqrt{\pi}\;\text{Gamma}[1+2\,\alpha]}\right)$$

$$P\,(-2-4\,\alpha,\,\alpha) = \frac{1}{4}+\frac{3\times 2^{-1+4\,a}\,(2+5\,a)\;\text{Gamma}\left[\frac{3}{2}+2\,a\right]}{(2+3\,a)\,\sqrt{\pi}\;\text{Gamma}[2+2\,a]}$$

$$P\,(-3-4\,\alpha,\,\alpha) = \frac{1}{4}+\frac{16^{\alpha}\,(36+\alpha\,(261+\alpha\,(517+4\,\alpha\,(97+25\,\alpha))))\;\text{Gamma}\left[\frac{3}{2}+2\,\alpha\right]}{\sqrt{\pi}\;(1+\alpha)\;(4+3\,\alpha)\;\text{Gamma}[4+2\,\alpha]}$$

$$P\,(-4-4\,\alpha,\,\alpha) =$$
$$\frac{1}{4}+\frac{4^{1+2\,\alpha}\,(600+\alpha\,(5810+\alpha\,(12\,177+\alpha\,(10\,169+20\,\alpha\,(186+25\,\alpha)))))\;\text{Gamma}\left[\frac{5}{2}+2\,\alpha\right]}{\sqrt{\pi}\;(4+3\,\alpha)\;(5+3\,\alpha)\;\text{Gamma}[6+2\,\alpha]}$$

$$P\,(-5-4\,\alpha,\,\alpha) =$$
$$\frac{1}{4}+\Big(16^{1+a}\,(3+a)\;(58\,800+a\,(864\,430+a\,(2\,885\,881+a\,(4\,390\,455+a\,(3\,663\,003+$$
$$a\,(1\,785\,405+2\,a\,(253\,653+50\,a\,(779+50\,a))))))))$$
$$\text{Gamma}\left[\frac{5}{2}+2\,a\right]\Big)\Big/\left((2+a)\;(5+3\,a)\;(7+3\,a)\;(8+3\,a)\;\sqrt{\pi}\;\text{Gamma}[2\;(4+a)]\right)$$

$$P\,(-6-4\,\alpha,\,\alpha) =$$
$$\frac{1}{4}+\Big(5\times 4^{3+2\,\alpha}\,(4+\alpha)\;(381\,024+\alpha\,(7\,556\,220+\alpha\,(26\,430\,672+\alpha\,(40\,827\,335+\alpha\,(34\,731\,485+$$
$$\alpha\,(17\,730\,421+5\,\alpha\,(1\,115\,269+2\,\alpha\,(105\,913+50\,\alpha\,(223+10\,\alpha)))))))))$$
$$\text{Gamma}\left[\frac{7}{2}+2\,\alpha\right]\Big)\Big/\left(3\,\sqrt{\pi}\;(2+\alpha)\;(7+3\,\alpha)\;(8+3\,\alpha)\;(10+3\,\alpha)\;\text{Gamma}[2\;(5+\alpha)]\right)$$

$$P\,(-7-4\,\alpha,\,\alpha) =$$
$$\frac{1}{4}+\Big(5\times 2^{7+4\,\alpha}\,(5+\alpha)\;(276\,623\,424+\alpha\,(7\,850\,387\,160+\alpha\,(35\,195\,799\,222+\alpha\,(72\,155\,175\,879+$$
$$\alpha\,(85\,815\,244\,768+\alpha\,(65\,555\,604\,072+\alpha\,(33\,830\,084\,228+$$
$$\alpha\,(12\,064\,972\,761+2\,\alpha\,(1\,490\,659\,419+8\,\alpha\,(31\,341\,498+$$
$$25\,\alpha\,(137\,012+25\,\alpha\,(351+10\,\alpha))))))))))))$$
$$\text{Gamma}\left[\frac{7}{2}+2\,\alpha\right]\Big)\Big/\Big(3\,\sqrt{\pi}\;(3+\alpha)\;(7+3\,\alpha)\;(8+3\,\alpha)\;(10+3\,\alpha)\;(11+3\,\alpha)$$
$$\text{Gamma}[2\;(6+\alpha)]\Big)$$

$$P\left(-8-4\alpha,\alpha\right)=\frac{1}{4}+\left(5\times 2^{11+4\alpha}(5+\alpha)(6+\alpha)\left(13356959616+\alpha\left(528863656464+\alpha\left(2457309996252+\alpha\left(5082252593676+\alpha\left(6056869914437+\alpha\left(4645534832462+\alpha\left(2427544767598+\alpha\left(890204059444+\alpha\left(231723009897+2\alpha\left(21317936217+20\alpha\left(135586447+50\alpha\left(226943+5\alpha\left(2249+50\alpha\right)\right)\right)\right)\right)\right)\right)\right)\right)\right)\right)\right)\right)\text{Gamma}\left[\frac{13}{2}+2\alpha\right]\right)\Big/\left(3\sqrt{\pi}(3+\alpha)(8+3\alpha)(10+3\alpha)(11+3\alpha)(13+3\alpha)(14+3\alpha)(9+4\alpha)(11+4\alpha)\,\text{Gamma}[2(7+\alpha)]\right)$$

$$P\left(-1/2-3\alpha,\alpha\right)=-\infty;$$
$$P\left(-3/2-3\alpha,\alpha\right)=-\infty;$$
$$P\left(-1/2-4\alpha,\alpha\right)=-\infty;$$
$$P\left(-3/2-4\alpha,\alpha\right)=-\infty$$

$$P\left(-1-3\alpha,\alpha\right)=\frac{3\,\text{Gamma}[3\alpha]\,\text{Gamma}[1+\alpha]+2\,\text{Gamma}[2\alpha]\,\text{Gamma}[1+2\alpha]}{2\,\alpha!\,(2\alpha)!\,\text{Gamma}[\alpha]}$$

$$P\left(-2-3\alpha,\alpha\right)=\left(-2\times 3^{\frac{3}{2}+3\alpha}(3+2\alpha)\left(-2+(-9+\alpha)\alpha(1+\alpha)\right)\text{Gamma}\left[\frac{2}{3}+\alpha\right]\text{Gamma}\left[\frac{4}{3}+\alpha\right]\text{Gamma}[3+\alpha]+4^{\alpha}\sqrt{\pi}\left(4+\alpha\left(8+\alpha+\alpha^2\right)\right)\text{Gamma}\left[\frac{3}{2}+\alpha\right]\text{Gamma}[5+2\alpha]\right)\Big/\left(2\pi(1+\alpha)\,\text{Gamma}[3+\alpha]\,\text{Gamma}[5+2\alpha]\right)$$
